# Supplementary material for: The Nitrogen Budget of Earth
Source: arXiv:1505.03813 source file (2015-05-14)
Supplement: Supplementary file 1 [file Read_Me_and_Supplemental_References.pdf]

# The Nitrogen Budget of Earth: Read me and Supplemental References

Included in the supplemental information are three files containing our data compilation. Each file is in csv format, and is comma-separated only. The first part of each file contains explanation of the abbreviations and column headings used in each file.

All data from minerals and rocks in the Earth are in the "Terrestrial N Data.csv" file. This file includes references, notes, sample names as used in original study, rock type, geologic setting, and year of study. Data include N and C isotopes and concentrations, as well as concentrations of elements observed to behave similarly to N: K, Rb, Lu, Yb, and Ar.

Data on N and C content of meteorites is in the "Meteorites.csv" file. It contains references, notes, individual meteorite names where known, as well as classification of each sample given as a class and clan. See Weisberg et al. (2006) for more detailed classification scheme; important classes for our study are "C" stands for carbonaceous chondrite, "E" for enstatite chondrite, and "I" for iron meteorites. We include N and C isotope and concentration data here.

The third file, "Experimental compilation.csv", contains our compilation of results from experimental petrologic studies concerning N. Listed are the parameters of the experimental run, including time of run, temperature, pressure, and oxygen fugacity. We calculate oxygen fugacity for experiments where it is not given as well as to determine ΔNNO (difference between sample oxygen fugacity and the fugacity at the NNO buffer at the same conditions) using the equation (Frost, 1991):

$$\log f_{O_2} = \mathrm{A/T + B + C(P-1)/(T)} \quad (1)$$

where T is temperature in K, P is pressure in bars, and constants A, B, and C are given in the file.

## References


Ahadnejad, V., Hirt, A. M., Valizadeh, M.-V., and Bokani, S. J. (2011). The ammonium content in the Malayer igneous and metamorphic rocks (Sanandaj-Sirjan Zone, Western Iran). *Geologica Carpathica*, 62(2):171–180.

Beaumont, V. and Robert, F. (1999). Nitrogen isotope ratios of kerogens in Precambrian cherts: a record of the evolution of atmosphere chemistry? *Precambrian Research*, 96(1):63–82.

Bebout, G., Agard, P., Kobayashi, K., Moriguti, T., and Nakamura, E. (2013). Devolatilization history and trace element mobility in deeply subducted sedimentary rocks: Evidence from Western Alps HP/UHP suites. *Chemical Geology*, 342:1–20.

Bebout, G., Cooper, D., Bradley, A. D., and Sadofsky, S. J. (1999a). Nitrogen-isotope record of fluid-rock interactions in the Skiddaw Auerole and granite, English Lake District. *American Mineralogist*, 84:1495–1505.

Bebout, G. and Fogel, M. (1992). Nitrogen-isotope compositions of metasedimentary rocks in the Catalina Schist, California: implications for metamorphic devolatilization history. *Geochimica et Cosmochimica Acta*, 56(7):2839–2849.

Bebout, G., Ryan, J., Leeman, W., and Bebout, A. (1999b). Fractionation of trace elements by subduction-zone metamorphism—effect of convergent-margin thermal evolution. *Earth and Planetary Science Letters*, 171(1):63–81.

Bebout, G. E. (1997). Nitrogen isotope tracers of high-temperature fluid-rock interactions: Case study of the Catalina Schist, California. *Earth and planetary science letters*, 151(1):77–90.

Boyd, S., Hall, A., and Pillinger, C. (1993). The measurement of $\delta^{15}$N in crustal rocks by static vacuum mass spectrometry: Application to the origin of the ammonium in the Cornubian batholith, southwest England. *Geochimica et Cosmochimica Acta*, 57(6):1339–1347.

Boyd, S. and Philippot, P. (1998). Precambrian ammonium biogeochemistry: a study of the Moine metasediments, Scotland. *Chemical Geology*, 144(3-4):257–268.

Bräuer, K., Kämpf, H., Niedermann, S., Strauch, G., and Weise, S. M. (2004). Evidence for a nitrogen flux directly derived from the European subcontinental mantle in the Western Eger Rift, central Europe. *Geochimica et cosmochimica acta*, 68(23):4935–4947.

Burgess, R., Cartigny, P., Harrison, D., Hobson, E., and Harris, J. (2009). Volatile composition of microinclusions in diamonds from the Panda kimberlite, Canada: implications for chemical and isotopic heterogeneity in the mantle. *Geochimica et Cosmochimica Acta*, 73(6):1779–1794.

Busigny, V., Ader, M., and Cartigny, P. (2005a). Quantification and isotopic analysis of nitrogen in rocks at the ppm level using sealed tube combustion technique: A prelude to the study of altered oceanic crust. *Chemical geology*, 223(4):249–258.

Busigny, V., Cartigny, P., and Philippot, P. (2011). Nitrogen isotopes in ophiolitic metagabbros: A re-evaluation of modern nitrogen fluxes in subduction zones and implication for the early earth atmosphere. *Geochimica et Cosmochimica Acta*, 75:7502–7521.

Busigny, V., Cartigny, P., Philippot, P., Ader, M., and Javoy, M. (2003). Massive recycling of nitrogen and other fluid-mobile elements (K, Rb, Cs, H) in a cold slab environment: evidence from HP to UHP oceanic metasediments of the Schistes Lustrés nappe (western Alps, Europe). *Earth and Planetary Science Letters*, 215(1):27–42.

Busigny, V., Laverne, C., and Bonifacie, M. (2005b). Nitrogen content and isotopic composition of oceanic crust at a superfast spreading ridge: A profile in altered basalts from ODP Site 1256, Leg 206. *Geochemistry, Geophysics, Geosystems*, 6(12):1–16.

Busigny, V., Lebeau, O., Ader, M., Krapež, B., and Bekker, A. (2013). Nitrogen cycle in the late archean ferruginous ocean. *Chemical Geology*, 362:115–130.

Cartigny, P., Boyd, S., Harris, J., and Javoy, M. (1997). Nitrogen isotopes in peridotitic diamonds from Fuxian, China: the mantle signature. *Terra Nova*, 9(4):175–179.

Cartigny, P., Harris, J., and Javoy, M. (2001). Diamond genesis, mantle fractionations and mantle nitrogen content: a study of $\delta^{13}$C–N concentrations in diamonds. *Earth and Planetary Science Letters*, 185(1):85–98.

Chicarelli, M. I., Hayes, J., Popp, B. N., Eckardt, C. B., and Maxwell, J. R. (1993). Carbon and nitrogen isotopic compositions of alkyl porphyrins from the triassic serpiano oil shale. *Geochimica et cosmochimica acta*, 57(6):1307–1311.

Cooper, D. and Bradley, A. (1990). The ammonium content of granites in the English Lake District. *Geological Magazine*, 127(06):579–586.

Cremonese, L., Shields-Zhou, G., Struck, U., Ling, H.-F., Och, L., Chen, X., and Li, D. (2013). Marine biogeochemical cycling during the early Cambrian constrained by a nitrogen and organic carbon isotope study of the Xiaotan section, South China. *Precambrian Research*, 225:148–165.

Cruz, M. D. R. (2011). $NH_4$-bearing micas in poly-metamorphic Alpujárride micaschists and gneisses from the central zone of the Betic Cordillera (Spain): tectono-metamorphic and crystal-chemical constraints. *Mineralogy and Petrology*, 101(3-4):225–244.

Dauphas, N. and Marty, B. (1999). Heavy nitrogen in carbonatites of the Kola Peninsula: A possible signature of the deep mantle. *Science*, 286(5449):2488–2490.

De Moor, J., Fischer, T., Sharp, Z., Hilton, D., Barry, P., Mangasini, F., and Ramirez, C. (2013). Gas chemistry and nitrogen isotope compositions of cold mantle gases from Rungwe Volcanic Province, southern Tanzania. *Chemical Geology*, 339:30–42.

Dixon, J. C., Campbell, S. W., and Durham, B. (2012). Geologic nitrogen and climate change in the geochemical budget of Kärkevagge, Swedish Lapland. *Geomorphology*, 167–168:70–76.

Drits, V. A., Lindgreen, H., and Salyn, A. L. (1997). Determination of the content and distribution of fixed ammonium in illite-smectite by x-ray diffraction: Application to north sea illite-smectite. *American Mineralogist*, 82(1):79–87.

Duit, W., Jansen, J. B. H., van Breemen, A., and Bos, A. (1986). Ammonium micas in metamorphic rocks as exemplified by Dome de l'Agout (France). *American Journal of Science*, 286(9):702–732.

Ekpo, B., Ibok, U., Essien, N., and Wehner, H. (2012). Geochemistry and organic petrography of cretaceous sediments of the calabar flank, southeastern, nigeria. *Marine and Petroleum Geology*, 35(1):252–268.

Elkins, L., Fischer, T., Hilton, D., Sharp, Z., McKnight, S., and Walker, J. (2006). Tracing nitrogen in volcanic and geothermal volatiles from the Nicaraguan volcanic front. *Geochimica et Cosmochimica Acta*, 70(20):5215–5235.

Exley, R., Boyd, S., Mattey, D., and Pillinger, C. (1987). Nitrogen isotope geochemistry of basaltic glasses: implications for mantle degassing and structure? *Earth and planetary science letters*, 81(2):163–174.

Fischer, T., Hilton, D., Zimmer, M., Shaw, A., Sharp, Z., and Walker, J. (2002). Subduction and recycling of nitrogen along the Central American margin. *Science*, 297(5584):1154–1157.

Franchi, I., Wright, I., and Pillinger, C. (1993). Constraints on the formation conditions of iron meteorites based on concentrations and isotopic compositions of nitrogen. *Geochimica et cosmochimica acta*, 57(13):3105–3121.

Frost, B. R. (1991). Introduction to oxygen fugacity and its petrologic importance. *Reviews in Mineralogy and Geochemistry*, 25(1):1–9.

Garvin, J., Buick, R., Anbar, A., Arnold, G., and Kaufman, A. (2009). Isotopic evidence for an aerobic nitrogen cycle in the latest Archean. *Science*, 323(5917):1045–1048.

Gibson, E., Carr, L., Gilmour, I., and Pillinger, C. (1986). Earth's atmosphere during the archean as seen from carbon and nitrogen isotopic analysis of sediments. In *Lunar and Planetary Institute Science Conference Abstracts*, volume 17, pages 258–259.

Gibson, E. and Moore, C. (1971). The distribution of total nitrogen in iron meteorites. *Geochimica et Cosmochimica Acta*, 35:877–890.

Gibson, E., Moore, C., and Lewis, C. (1971). Total nitrogen and carbon abundances in carbonaceous chondrites. *Geochimica et Cosmochimica Acta*, 35:599–604.

Glasmacher, U., Zentilli, M., and Ryan, R. (2003). Nitrogen distribution in lower palaeozoic slates/phyllites of the meguma supergroup, nova scotia, canada: implications for au and zn–pb mineralisation and exploration. *Chemical geology*, 194(4):297–329.

Godfrey, L. and Falkowski, P. (2009). The cycling and redox state of nitrogen in the Archaean ocean. *Nature Geoscience*, 2(10):725–729.

Godfrey, L., Poulton, S., Bebout, G., and Fralick, P. (2013). Stability of the nitrogen cycle during development of sulfidic water in the redox-stratified late Paleoproterozoic Ocean. *Geology*, 41:655–658.

Grady, M. M. and Pillinger, C. (1986). Carbon isotope relationships in winonaites and forsterite chondrites. *Geochimica et Cosmochimica Acta*, 50:255–263.

Grady, M. M. and Wright, I. P. (2003). Elemental and isotopic abundances of carbon and nitrogen in meteorites. *Space Science Reviews*, 106(1):231–248.

Greenfield, L. (1988). 3.2 Forms of Nitrogen in Beacon Sandstone Rocks Containing Endolithic Microbial Communities in Southern Victoria Land, Antarctica. *Polarforschung*, 58(2/3):211–218.

Greenfield, L. (1991). Fixed ammonium in antarctic rocks and soils and a possible cause of underestimation. *Soil Biology and Biochemistry*, 23(4):397–399.

Haendel, D., Mühle, K., Nitzsche, H.-M., Stiehl, G., and Wand, U. (1986). Isotopic variations of the fixed nitrogen in metamorphic rocks. *Geochimica et cosmochimica Acta*, 50(5):749–758.

Halama, R., Bebout, G., John, T., and Scambelluri, M. (2012). Nitrogen recycling in subducted mantle rocks and implications for the global nitrogen cycle. *International Journal of Earth Sciences*, pages 1–19.

Halama, R., Bebout, G. E., John, T., and Schenk, V. (2010). Nitrogen recycling in subducted oceanic lithosphere: The record in high-and ultrahigh-pressure metabasaltic rocks. *Geochimica et Cosmochimica Acta*, 74(5):1636–1652.

Halbout, J., Mayeda, T., and Clayton, R. N. (1986). Carbon isotopes and light element abundances in carbonaceous chondrites. *Earth and Planetary Science Letters*, 80:1–18.

Hall, A. (1987). The ammonium content of Caledonian granites. *Journal of the Geological Society*, 144(4):671–674.

Hall, A. (1988). The distribution of ammonium in granites from South-West England. *Journal of the Geological Society*, 145(1):37–41.

Hall, A. (1999). Ammonium in granites and its petrogenetic significance. *Earth-Science Reviews*, 45(3):145–165.

Hall, A., Bencini, A., and Poli, G. (1991). Magmatic and hydrothermal ammonium in granites of the Tuscan magmatic province, Italy. *Geochimica et Cosmochimica Acta*, 55(12):3657–3664.

Hall, A., Pereira, M., and Bea, F. (1996). The abundance of ammonium in the granites of central spain, and the behaviour of the ammonium ion during anatexis and fractional crystallization. *Mineralogy and Petrology*, 56(1-2):105–123.

Hashizume, K. and Sugiura, N. (1995). Nitrogen isotopes in bulk ordinary chondrites. *Geochimica et cosmochimica acta*, 59(19):4057–4069.

Hayes, J., Wedeking, K., and Kaplan, I. (1983). Precambrian organic geochemistry-preservation of the record.

Hoering, T. (1955). Variations of nitrogen-15 abundance in naturally occurring substances. *Science*, 122(3182):1233–1234.

Holloway, J. M., Dahlgren, R. A., and Casey, W. H. (2001). Nitrogen release from rock and soil under simulated field conditions. *Chemical Geology*, 174(4):403–414.

Honma, H. (1996). High ammonium contents in the 3800 Ma isua supracrustal rocks, central west greenland. *Geochimica et cosmochimica acta*, 60(12):2173–2178.

Imbus, S., Macko, S., Douglas Elmore, R., and Engel, M. (1992). Stable isotope (C, S, N) and molecular studies on the Precambrian Nonesuch Shale (Wisconsin-Michigan, USA): evidence for differential preservation rates, depositional environment and hydrothermal influence. *Chemical Geology: Isotope Geoscience section*, 101(3):255–281.

Itihara, Y. and Honma, H. (1979). Ammonium in biotite from metamorphic and granitic rocks of Japan. *Geochimica et Cosmochimica Acta*, 43(4):503–509.

Itihara, Y. and Suwa, K. (1985). Ammonium contents of biotites from precambrian rocks in finland: The significance of nh¡ sub¿ 4¡/sub¿¡ sup¿+¡/sup¿ as a possible chemical fossil. *Geochimica et Cosmochimica Acta*, 49(1):145–151.

Itihara, Y., Suwa, K., and Hoshino, M. (1986). Organic matter in the Kavirondian sedimentary rocks of Archaean period in Kenya. *Geochemical Journal*, 20(4):201–207.

Itihara, Y. and Tainosho, Y. (1989). Ammonium and insoluble nitrogen in precambrian rock from the Gawler Craton, Australia: Inference of life activity. *Journal of the Geological Society of Japan*, 95(6):439–445.

Ivanova, M., Kononkova, N., Krot, A., Greenwood, R., Franchi, I. A., Verchovsky, A., Trieloff, M., Korochantseva, E., and Brandstätter, F. (2008). The Isheyevo meteorite: Mineralogy, petrology, bulk chemistry, oxygen, nitrogen, carbon isotopic compositions, and $^{40}$Ar-$^{39}$Ar ages. *Meteoritics and Planetary Science*, 43(5):915–940.

Jenkyns, H. C., Gröcke, D. R., and Hesselbo, S. P. (2001). Nitrogen isotope evidence for water mass denitrification during the early Toarcian (Jurassic) oceanic anoxic event. *Paleoceanography*, 16(6):593–603.

Jia, Y. (2006). Nitrogen isotope fractionations during progressive metamorphism: A case study from the Paleozoic Cooma metasedimentary complex, southeastern Australia. *Geochimica et cosmochimica acta*, 70(20):5201–5214.

Jia, Y. and Kerrich, R. (1999). Nitrogen isotope systematics of mesothermal lode gold deposits: Metamorphic, granitic, meteoric water, or mantle origin? *Geology*, 27(11):1051–1054.

Jia, Y. and Kerrich, R. (2000). Giant quartz vein systems in accretionary orogenic belts: the evidence for a metamorphic fluid origin from $\delta^{15}$N $\delta^{13}$C studies. *Earth and Planetary Science Letters*, 184(1):211–224.

Jia, Y., Kerrich, R., Gupta, A., and Fyfe, W. (2003). $^{15}$N–enriched Gondwana lamproites, eastern India: crustal N in the mantle source. *Earth and Planetary Science Letters*, 215(1):43–56.

Kadik, A., Kurovskaya, N., Ignat'ev, Y., Kononkova, N., Koltashev, V., and Plotnichenko, V. (2011). Influence of oxygen fugacity on the solubility of nitrogen, carbon, and hydrogen in FeO-$Na_2O$-$SiO_2$-$Al_2O_3$ melts in equilibrium with metallic iron at 1.5 GPa and 1400°C. *Geochemistry International*, 49(5):429–438.

Kao, S. and Liu, K. (2000). Stable carbon and nitrogen isotope systematics in a human-disturbed watershed (lanyang-hsi) in taiwan and the estimation of biogenic particulate organic carbon and nitrogen fluxes. *Global Biogeochemical Cycles*, 14(1):189–198.

Kerrich, R., Jia, Y., Manikyamba, C., and Naqvi, S. (2006). Secular variations of N-isotopes in terrestrial reservoirs and ore deposits. *Evolution of Early Earth's Atmosphere, Hydrosphere, And Biosphere: Constraints from Ore Deposits*, 198:81–104.

Kerridge, J. (1985). Carbon, hydrogen and nitrogen in carbonaceous chondrites: Abundances and isotopic compositions in bulk samples. *Geochimica et Cosmochimica Acta*, 49:1707–1714.

Kung, C. and Clayton, R. N. (1978). Nitrogen abundances and isotopic compositions in stony meteorites. *Earth and Planetary Science Letters*, 38:421–435.

Li, L., Bebout, G., and Idleman, B. (2007). Nitrogen concentration and $\delta^{15}$N of altered oceanic crust obtained on ODP Legs 129 and 185: Insights into alteration-related nitrogen enrichment and the nitrogen subduction budget. *Geochimica et Cosmochimica Acta*, 71:2344–2360.

Li, L. and Bebout, G. E. (2005). Carbon and nitrogen geochemistry of sediments in the Central American convergent margin: Insights regarding subduction input fluxes, diagenesis, and paleoproductivity. *Journal of Geophysical Research: Solid Earth (1978–2012)*, 110(B11).

Li, L., Zheng, Y.-F., Cartigny, P., and Li, J. (2014). Anomalous nitrogen isotopes in ultrahigh-pressure metamorphic rocks from the Sulu orogenic belt: Effect of abiotic nitrogen reduction during fluid–rock interaction. *Earth and Planetary Science Letters*, 403:67–78.

Li, Y., Huang, R., Wiedenbeck, M., and Keppler, H. (2015). Nitrogen distribution between aqueous fluids and silicate melts. *Earth and Planetary Science Letters*, 411:218–228.

Li, Y., Wiedenbeck, M., Shcheka, S., and Keppler, H. (2013). Nitrogen solubility in upper mantle minerals. *Earth and Planetary Science Letters*, 377:311–323.

Libourel, G., Marty, B., and Humbert, F. (2003). Nitrogen solubility in basaltic melt. Part I. Effect of oxygen fugacity. *Geochimica et Cosmochimica Acta*, 67(21):4123–4135.

Marty, B. (1995). Nitrogen content of the mantle inferred from $N_2$–Ar correlation in oceanic basalts. *Nature*, 377(6547):326–329.

Marty, B. and Dauphas, N. (2003). The nitrogen record of crust–mantle interaction and mantle convection from Archean to present. *Earth and Planetary Science Letters*, 206(3):397–410.

Marty, B. and Humbert, F. (1997). Nitrogen and argon isotopes in oceanic basalts. *Earth and Planetary Science Letters*, 152(1):101–112.

Marty, B. and Zimmermann, L. (1999). Volatiles (He, C, N, Ar) in mid-ocean ridge basalts: Assesment of shallow-level fractionation and characterization of source composition. *Geochimica et Cosmochimica Acta*, 63(21):3619–3633.

Mason, B. (1979). Data of geochemistry sixth edition. *Geological Survey Professional Paper*, 440-B-1(Chapter B. Cosmochemistry).

Mathew, K. and Marti, K. (2001). Lunar nitrogen: indigenous signature and cosmic-ray production rate. *Earth and Planetary Science Letters*, 184:659–669.

Mathew, K., Marty, B., Marti, K., and Zimmermann, L. (2003). Volatiles (nitrogen, noble gases) in recently discovered SNC meteorites, extinct radioactivities and evolution. *Earth and Planetary Science Letters*, 214:27–42.

Mathew, K., Palma, R., Marti, K., and Lavielle, B. (2000). Isotopic signatures and origin of nitrogen in IIE and IVA iron meteorites. *Geochimica et Cosmochimica Acta*, 64(3):545–557.

Matsumoto, T., Pinti, D., Matsuda, J., and Umino, S. (2002). Recycled noble gas and nitrogen in the subcontinental lithospheric mantle: Implications from N–He–Ar in fluid inclusions of SE Australian xenoliths. *Geochemical Journal of Japan*, 36(3):209–218.

Mingram, B. and Bräuer, K. (2001). Ammonium concentration and nitrogen isotope composition in metasedimentary rocks from different tectonometamorphic units of the European Variscan belt. *Geochimica et Cosmochimica Acta*, 65(2):273–287.

Mohapatra, R., Harrison, D., Ott, U., Gilmour, J., and Trieloff, M. (2009). Noble gas and nitrogen isotopic components in Oceanic Island Basalts. *Chemical Geology*, 266(1):29–37.

Mohapatra, R. and Murty, S. (2003). Precurors of Mars: Constraints from nitrogen and oxygen isotopic compositions of martioan meteorites. *Meteoritics and Planetary Science*, 38(2):225–241.

Morford, S. L., Houlton, B. Z., and Dahlgren, R. A. (2011). Increased forest ecosystem carbon and nitrogen storage from nitrogen rich bedrock. *Nature*, 477(7362):78–81.

Mysen, B. O. and Fogel, M. L. (2010). Nitrogen and hydrogen isotope compositions and solubility in silicate melts in equilibrium with reduced (N+ H)-bearing fluids at high pressure and temperature: Effects of melt structure. *American Mineralogist*, 95(7):987–999.

Mysen, B. O., Yamashita, S., and Chertkova, N. (2008). Solubility and solution mechanisms of NOH volatiles in silicate melts at high pressure and temperature-amine groups and hydrogen fugacity. *Am. Mineral*, 93:1760–1770.

Nishio, Y., Ishii, T., Gamo, T., and Sano, Y. (1999). Volatile element isotopic systematics of the Rodrigues Triple Junction Indian Ocean MORB: implications for mantle heterogeneity. *Earth and Planetary Science Letters*, 170(3):241–253.

Palot, M., Cartigny, P., Harris, J., Kaminsky, F., and Stachel, T. (2012). Evidence for deep mantle convection and primordial heterogeneity from nitrogen and carbon stable isotopes in diamond. *Earth and Planetary Science Letters*, 357:179–193.

Palya, A. P., Buick, I. S., and Bebout, G. E. (2011). Storage and mobility of nitrogen in the continental crust: Evidence from partially melted metasedimentary rocks, Mt. Stafford, Australia. *Chemical Geology*, 281(3):211–226.

Papineau, D., Mojzsis, S., Karhu, J., and Marty, B. (2005). Nitrogen isotopic composition of ammoniated phyllosilicates: case studies from Precambrian metamorphosed sedimentary rocks. *Chemical Geology*, 216(1):37–58.

Papineau, D., Purohit, R., Goldberg, T., Pi, D., Shields, G. A., Bhu, H., Steele, A., and Fogel, M. L. (2009). High primary productivity and nitrogen cycling after the Paleoproterozoic phosphogenic event in the Aravalli Supergroup, India. *Precambrian Research*, 171(1):37–56.

Pearson, V., Sephton, M. A., Franchi, I., Gibson, J., and Gilmour, I. (2006). Carbon and nitrogen in carbonaceous chondrites: Elemental abundances and stable isotopic compositions. *Meteoritics and Planetary Science*, 41(12):1899–1918.

Pepin, R. O. and Becker, R. H. (1982). Nitrogen isotopes in iron meteorites. *Meteoritics*, 17:269.

Peters, K., Sweeney, R., and Kaplan, I. (1978). Correlation of carbon and nitrogen stable isotope ratios in sedimentary organic matter. *Limnololgy and Oceanography*, 23(4):598–604.

Philippot, P., Busigny, V., Scambelluri, M., and Cartigny, P. (2007). Oxygen and nitrogen isotopes as tracers of fluid activities in serpentinites and metasediments during subduction. *Mineralogy and Petrology*, 91(1-2):11–24.

Pinti, D., Hashizume, K., and Matsuda, J. (2001). Nitrogen and argon signatures in 3.8 to 2.8 Ga metasediments: Clues on the chemical state of the Archean ocean and the deep biosphere. *Geochimica et Cosmochimica Acta*, 65(14):2301–2315.

Pitcairn, I., Teagle, D., Kerrich, R., Craw, D., and Brewer, T. (2005). The behavior of nitrogen and nitrogen isotopes during metamorphism and mineralization: evidence from the Otago and Alpine Schists, New Zealand. *Earth and Planetary Science Letters*, 233(1):229–246.

Plessen, B., Harlov, D. E., Henry, D., and Guidotti, C. V. (2010). Ammonium loss and nitrogen isotopic fractionation in biotite as a function of metamorphic grade in metapelites from western Maine, USA. *Geochimica et Cosmochimica Acta*, 74(16):4759–4771.

Ponganis, K. and Marti, K. (2007). Nitrogen components in IAB/IIICD iron meteorites. *Meteoritics and Planetary Science*, 42(3):331–346.

Pontes, F. V., Carneiro, M. C., Vaitsman, D. S., da Rocha, G. P., da Silva, L. I., Neto, A. A., and Monteiro, M. I. C. (2009). A simplified version of the total kjeldahl nitrogen method using an ammonia extraction ultrasound-assisted purge-and-trap system and ion chromatography for analyses of geological samples. *Analytica Chimica Acta*, 632(2):284–288.

Power, J., Bond, J., Sandoval, F., and Willis, W. (1974). Nitrification in paleocene shale. *Science*, 183(4129):1077–1079.

Prombo, C. A. and Clayton, R. N. (1993). Nitrogen isotopic compositions of iron meteorites. *Geochimica et cosmochimica acta*, 57(15):3749–3761.

Quan, T., van de Schootbrugge, B., Field, M., Rosenthal, Y., and Falkowski, P. (2008). Nitrogen isotope and trace metal analyses from the Mingolsheim core (Germany): Evidence for redox variations across the Triassic-Jurassic boundary. *Global Biogeochemical Cycles*, 22(2):GB2014.

Rau, G., Arthur, M., and Dean, W. (1987). $^{15}N/^{14}N$ variations in Cretaceous Atlantic sedimentary sequences: implication for past changes in marine nitrogen biogeochemistry. *Earth and Planetary Science Letters*, 82(3):269–279.

Rigby, D. and Batts, B. (1986). The isotopic composition of nitrogen in Australian coals and oil shales. *Chemical Geology: Isotope Geoscience section*, 58(3):273–282.

Robert, F. and Epstein, S. (1982). The concentration and isotopic composition of hydrogen, carbon and nitrogen in carbonaceous meteorites. *Geochimica et Cosmochimica Acta*, 46:81–95.

Roskosz, M., Bouhifd, M., Jephcoat, A., Marty, B., and Mysen, B. (2013). Nitrogen solubility in molten metal and silicate at high pressure and temperature. *Geochimica et Cosmochimica Acta*, 121:15–28.

Roskosz, M., Mysen, B. O., and Cody, G. D. (2006). Dual speciation of nitrogen in silicate melts at high pressure and temperature: an experimental study. *Geochimica et Cosmochimica Acta*, 70(11):2902–2918.

Roulleau, E., Pinti, D., Stevenson, R., Takahata, N., Sano, Y., and Pitre, F. (2012). N, Ar and Pb isotopic co-variations in magmatic minerals: Discriminating fractionation processes from magmatic sources in Monteregian Hills, Québec, Canada. *Chemical Geology*.

Sadofsky, S. J. and Bebout, G. E. (2000). Ammonium partitioning and nitrogen-isotope fractionation among coexisting micas during high-temperature fluid-rock interactions: Examples from the New England Appalachians. *Geochimica et Cosmochimica Acta*, 64(16):2835–2849.

Sadofsky, S. J. and Bebout, G. E. (2003). Record of forearc devolatilization in low-T, high-P/T metasedimentary suites: Significance for models of convergent margin chemical cycling. *Geochemistry, Geophysics, Geosystems*, 4(4).

Sadofsky, S. J. and Bebout, G. E. (2004). Nitrogen geochemistry of subducting sediments: New results from the Izu-Bonin-Mariana margin and insights regarding global nitrogen subduction. *Geochemistry, Geophysics, Geosystems*, 5(3).

Sakai, H., Des Marais, D., Ueda, A., and Moore, J. (1984). Concentrations and isotope ratios of carbon, nitrogen and sulfur in ocean-floor basalts. *Geochimica et Cosmochimica Acta*, 48(12):2433–2441.

Sano, Y. and Pillinger, C. (1990). Nitrogen isotopes and $N_2$/Ar ratios in cherts: an attempt to measure time evolution of atmospheric $\delta^{15}$N value. *Geochem. J*, 24:315–325.

Sano, Y., Takahata, N., Nishio, Y., Fischer, T., and Williams, S. (2001). Volcanic flux of nitrogen from the Earth. *Chemical geology*, 171(3):263–271.

Sano, Y., Takahata, N., Nishio, Y., and Marty, B. (1998). Nitrogen recycling in subduction zones. *Geophysical research letters*, 25(13):2289–2292.

Schroeder, P. and McLain, A. (1998). Illite-smectites and the influence of burial diagenesis on the geochemical cycling of nitrogen. *Clay Minerals*, 33(4):539–546.

Schulze, D. J., Coopersmith, H. G., Harte, B., and Pizzolato, L.-A. (2008). Mineral inclusions in diamonds from the Kelsey Lake Mine, Colorado, USA: Depleted Archean mantle beneath the Proterozoic Yavapai province. *Geochimica et Cosmochimica Acta*, 72(6):1685–1695.

Sephton, M. A., Amor, K., Franchi, I. A., Wignall, P. B., Newton, R., and Zonneveld, J.-P. (2002). Carbon and nitrogen isotope disturbances and an end-Norian (Late Triassic) extinction event. *Geology*, 30(12):1119–1122.

Sephton, M. A., Verchovsky, A., Bland, P., Gilmour, I., Grady, M. M., and Wright, I. (2003). Investigating the variatuibs in carbon and nitrogen isotopes in carbonaceous chondrites. *Geochimica et Cosmochimica Acta*, 67(11):2093–2108.

Smelov, A., Shatsky, V., Ragozin, A., Reutskii, V., and Molotkov, A. (2012). Diamondiferous archean rocks of the olondo greenstone belt (*western Aldan–Stanovoy shield*). *Russian Geology and Geophysics*, 53(10):1012–1022.

Stiehl, G. and Lehmann, M. (1980). Isotopenvariationen des stickstoffs humoser und bituminöser natürlicher organischer substanzen. *Geochimica et Cosmochimica Acta*, 44(11):1737–1746.

Sugiura, N. (1998). Ion probe measurements of carbon and nitrogen in iron meteorites. *Meteoritics and Planetary Science*, 33:393–409.

Sugiura, N., Kiyota, K., and Hashizume, K. (1998). Nitrogen components in primitive ordinary chondrites. *Meteoritics and Planetary Science*, 33:463–482.

Sugiura, N. and Zashu, S. (1995). Nitrogen isotopic composition of CK chondrites. *Meteoritics*, 30:430–435.

Sullivan, P. J., Sposito, G., Strathouse, S., and Hansen, C. L. (1979). *Geologic nitrogen and the occurrence of high nitrate soils in the western San Joaquin Valley, California.* University of California, Division of Agriculture and Natural Resources.

Svensen, H., Bebout, G., Kronz, A., Li, L., Planke, S., Chevallier, L., and Jamtveit, B. (2008). Nitrogen geochemistry as a tracer of fluid flow in a hydrothermal vent complex in the karoo basin, south africa. *Geochimica et Cosmochimica Acta*, 72(20):4929–4947.

Tappert, R., Stachel, T., Harris, J. W., Muehlenbachs, K., Ludwig, T., and Brey, G. P. (2005). Diamonds from jagersfontein (south africa): messengers from the sublithospheric mantle. *Contributions to Mineralogy and Petrology*, 150(5):505–522.

Thomazo, C., Ader, M., and Philippot, P. (2011). Extreme $^{15}$N-enrichments in 2.72-Gyr-old sediments: evidence for a turning point in the nitrogen cycle. *Geobiology*, 9(2):107–120.

Ueno, Y., Yoshioka, H., Maruyama, S., and Isozaki, Y. (2004). Carbon isotopes and petrography of kerogens in $\sim$ 3.5–Ga hydrothermal silica dikes in the North Pole area, Western Australia. *Geochimica et Cosmochimica Acta*, 68(3):573–589.

van Zuilen, M. A., Mathew, K., Wopenka, B., Lepland, A., Marti, K., and Arrhenius, G. (2005). Nitrogen and argon isotopic signatures in graphite from the 3.8-ga-old isua supracrustal belt, southern west greenland. In *Lunar and Planetary Institute Science Conference Abstracts*, volume 69, pages 1241–1252. Elsevier.

Visser, D. (1993). The metamorphic evolution of the Bamble sector, south Norway: A paragenetic and mineral chemical study of cordierite-orthoamphibole-bearing rocks with special reference to borosilicate-bearing mineral assemblages. *Geologica Ultraiectina*, 103:1–159.

Watanabe, Y., Naraoka, H., Wronkiewicz, D., Condie, K., and Ohmoto, H. (1997). Carbon, nitrogen, and sulfur geochemistry of Archean and Proterozoic shales from the Kaapvaal Craton, South Africa. *Geochimica et Cosmochimica Acta*, 61(16):3441–3459.

Weisberg, M. K., McCoy, T. J., and Krot, A. N. (2006). Systematics and evaluation of meteorite classification. *Meteorites and the early solar system II*, 19.

Westerlund, K., Shirey, S., Richardson, S., Carlson, R., Gurney, J., and Harris, J. (2006). A subduction wedge origin for Paleoarchean peridotitic diamonds and harzburgites from the Panda kimberlite, Slave craton: evidence from Re–Os isotope systematics. *Contributions to Mineralogy and Petrology*, 152(3):275–294.

Williams, L., Wilcoxon, B., Ferrell, R., and Sassen, R. (1992). Diagenesis of ammonium during hydrocarbon maturation and migration, wilcox group, louisiana, usa. *Applied Geochemistry*, 7(2):123–134.

Williams, L. B., Ferrell, R. E., Hutcheon, I., Bakel, A. J., Walsh, M. M., and Krouse, H. R. (1995). Nitrogen isotope geochemistry of organic matter and minerals during diagenesis and hydrocarbon migration. *Geochimica et Cosmochimica Acta*, 59(4):765–779.

Williams, L. B. and Ferrell Jr, R. (1991). Ammonium substitution in illite during maturation of organic matter. *Clays and Clay Minerals*, 39(4):400–408.

Yamaguchi, K. (2002). *Geochemistry of Archean–Paleoproterozoic black shales: The early evolution of the atmosphere, oceans, and biosphere*. PhD thesis, The Pennsylvania State University.

Yokochi, R., Marty, B., Chazot, G., and Burnard, P. (2009). Nitrogen in peridotite xenoliths: Lithophile behavior and magmatic isotope fractionation. *Geochimica et Cosmochimica Acta*, 73(16):4843–4861.

Yui, T.-F., Kao, S.-J., and Wu, T.-W. (2009). Nitrogen and N-isotope variation during low-grade metamorphism of the Taiwan mountain belt. *Geochemical Journal*, 43(1):15–27.
